# Supplementary material for: Complexity of Discrete Energy Minimization Problems
Source: arXiv:1607.08905 source file (2016-07-29)
Supplement: Supplementary file 1 [file supplement.tex]

\section{Supplementary Material (To Be Moved to Another Project}

For multi-label problems~\citet{Ishikawa03} proposed a reduction to minimum cut for problems with convex interactions, \ie, where $f_{uv}(x_u,x_v) = g_{uv}(x_u - x_v)$ and $g_{uv}$ is convex. % while~\cite{Hochbaum-2001-MRF} proposed directly an efficient algorithm for the case of .
Ordered multi-label submodular
It is worth noting that in case when unary terms are convex as well the problem can be solved even more efficiently~\cite{Hochbaum-2001-MRF,Kolmogorov05primal-dualalgorithm}. %The construction by~\citet{Hochbaum-2001-MRF} 
The same reduction~\cite{Ishikawa03} remains correct for a more general class of submodular multi-label problems. % possible wrong citation \cite{Ishikawa03}
In modern terminology, component-wise minimum $x \wedge y$ and component-wise maximum $x \vee y$ of labelings $x$, $y$ are introduced. These operations define a lattice on the set of labelings. The function $f$ is called {\em submodular} on the lattice if $f(x \vee y) + f(x \wedge y) \leq f(x) + f(y)$. In the pairwise case, the condition becomes equivalent to that each $f_{uv}$ is submodular.
Submodularity depends on the order of labels. \citet{DSchlesinger-07-permuted} proposed an algorithm to find a reordering in which the problem is submodular if one exists.
 %Generalizing on operation $\vee$ and $\wedge$, a class of bisubmodular 
%\revisit
% less relevant move to the appendix
There have been many generalizations of multi-label submodular functions proposed which until the following result has been finally established:
 \begin{theorem}[\citet{Thapper-12,Thapper-13}]
 Let $D$ be an arbitrary finite set and $L$ a class of functions from $D$ to $\Rationals$. Let $C_L$ be the class of instances with functions from $L$.
 \begin{enumerate}
 \item Either every $f \in L$ satisfies a certain algebraic condition
 and Basic LP relaxation (BLP) solves every instance from $C_L$,
 \item or $C_L$ encodes MAXCUT and hence is NP-hard.
 \end{enumerate}
 \end{theorem}
This result covers the following special cases (see~\cite{Thapper-13}): symmetric tournament pair, submodularity on arbitrary trees, submodularity on arbitrary lattices, skew bisubmodularity, bisubmodularity on arbitrary domains. It follows that all tractable problems with interaction restrictions has been characterized. Moreover, if the problem is tractable it can be solved by an LP relaxation technique.
